# Supplementary material for: Order-Reduction Abstractions for Safety Verification of High-Dimensional Linear Systems
Source: arXiv:1602.06417 source file (2016-02-20)
Supplement: Supplementary file 1 [file appendix_result.tex]

\subsection{Appendix: Additional Experimental Results}
\applabel{Appendix_result}
In this appendix, we describe additional experimental results using our approach.

%\paragraph*{Periodically switched synchronous motor position control system initial conditions}
%%
%\begin{table}[t]%
	%\tiny%
	%\centering%
	%\begin{tabular}{|l|l|}
  %\hline
  %Vector  & Value \\
	%\hline
  %$lb^1$  & [-0.002~~0~~0~~0~~-0.001~~0~~0~~0$]^T$  \\
  %$ub^1$  & [0.0025~~0~~0~~0~~0.002~~0~~0~~0$]^T$  \\
	%$lb^2$  & [-0.001~~0~~0~~0~~-0.002~~0~~0~~0$]^T$  \\
  %$ub^2$  & [0.001~~0~~0~~0~~0.003~~0~~0~~0$]^T$  \\
  %$lb^1_r$  & [-0.1373e-03~~-0.5137e-03~~-0.0586e-03~~-0.2277e-03~~-0.2235e-03$]^T$  \\
  %$ub^1_r$  & [0.1323e-03~~0.5332e-03~~0.0930e-03~~0.3610e-03~~0.2320e-03$]^T$  \\
	%$lb^2_r$  & [-0.1211e-03~~-0.3684e-03~~-0.0687e-03~~-0.2666e-03~~-0.1603e-03$]^T$  \\
  %$ub^2_r$  & [0.0949e-03~~0.4703e-03~~0.0949e-03~~0.3684e-03~~0.2046e-03$]^T$  \\
  %\hline
%\end{tabular}
	%\caption{Initial condition vectors of the periodically synchronous motor control system and its 5th-order output abstraction.}%
	%\tablabel{4}% % pleaes use descriptive labels instead of numbers...
	%\vspace{-2em}
%\end{table}

\paragraph*{Building model (BM)}
We consider the model of Los Angeles University Hospital with 8 floors each of which has 3 degrees of freedom~\cite{Antoulas01asurvey}.
The full order state space model of this system (denoted by $M_{48}$) has 48 state variables in which we are mostly interested in the twenty-fifth state $x_{25}(t)$ which is the motion of the first coordinate.
We do not present the system's matrices here due to their large sizes, but they are included in the supplementary materials.

Assume that the initial set of the system is as follows:
\begin{equation*}
X_0 = \{x \in \mathbb{R}^{48} | -0.0001 \leq x_{25} \leq 0.0001, x_i = 0,~ \forall i\neq 25\}.
\end{equation*}

The safety requirement of the system is that under a 1-radian step disturbance at the input and the above initial condition $X_0$, the output $y = x_{25}(t)$ is not larger than $p_{max} = 0.0015$ and not smaller than $p_{min} = -0.0015$.
Formally, the safety specification of the system can be written as $S(M_{48}) = \{y \in \mathbb{R}^{1}|~-0.0015 \leq y \leq 0.0015\}$.
The verification problem is to check whether $M_{48} \models S(M_{48})$.

To verify whether $M_{48}$ satisfies its safety specification, we can use an output abstraction of the original system.
Let's consider using the 10-order output abstraction $M_{10}^{\delta}$.
The error bounds between the output abstraction and the original system are presented in~\tabref{tab:1}.
It should be emphasized again that the bound of $e_1$ corresponding to zero-input response is normally hardly determined via simulation since we can not simulate all vertices of the initial set.
With our method, a tight bound of $e_1$ is easily obtained.
As shown in the table, the theoretical bound of $e_2$ corresponding to zero-state response is much larger than its actual bound determined via simulation.
Consequently, the theoretical error bound $\delta$ is $0.0050$ which is even larger than the safety requirement $p_{max} = 0.0015$.
Therefore, in this case, we cannot use this theoretical error bound.
Instead, the tighter bound $\delta = 3.7219e-04 $ is used for verification process.

The initial set of $M^{\delta}_{10}$ is transformed from the initial set of the original system $M_{48}$ as follows $X_{0}(M^{\delta}_{10}) = \{x_r \in \mathbb{R}^{10},~y_r \in \mathbb{R}^{1} |~lb_{r}(i) \leq x_r(i) \leq ub_{r}(i),~ 1\leq i \leq 10 \wedge a \leq y_r \leq b\}$, where $lb_r,~ub_r,~a,~b$ are given in \tabref{tab:2}.

\begin{table}
	\centering
	\begin{tabular}{|l|l|l|}
  \hline
  Error  & Theoretical bound & Simulation-based actual bound \\
	\hline
  $e_{1}$  & 2.3586e-04 & --- \\
  $e_{2}$  & 0.0047 & 1.3633e-04  \\
  $\delta$ & 0.0050 & 3.7219e-04 \\
  \hline
\end{tabular}
	\caption{The error bound between the full order BM system $M_{48}$ and its 10-order output abstraction $M_{10}^{\delta}$.}
	\tablabel{tab:1}
\end{table}

\begin{table}
	\centering
	\tiny
	\begin{tabular}{|l|l|}
  \hline
  Vector  & Value \\
	\hline
  $lb_r$  & [-4.4771e-05~~-4.7113e-04~~-5.0817e-06~~-4.5431e-04~~-2.5589e-05~~ \\
	        &  -3.4480e-04~~-1.5641e-04~~-6.8385e-05~~-8.2134e-05~~-8.7017e-05$]^T$  \\
  $ub_r$  & [2.2385e-04~~0.0024~~2.5409e-05~~0.0023~~1.2794e-04~~ \\
	        &  0.0017~~7.8206e-04~~3.4193e-04~~4.1067e-04~~4.3509e-04$]^T$ \\
  $a$     & -8.1277e-05  \\
	$b$     &  8.1278e-05  \\
  \hline
\end{tabular}
	\caption{Transformed initial condition of BM's 10-order output abstraction $M_{10}^{\delta}$.}
	\tablabel{tab:2}
\end{table}

Now, instead of verifying the original system $M_{48}$ with a high computation cost, we will verify whether the 10-order output abstraction satisfies its transformed safety specification, i.e. we check whether $M^{\delta}_{10} \models S(M^{\delta}_{10})$, where $ S(M^{\delta}_{10}) = \{y_r \in \mathbb{R}^1| ~-0.00112781 = p_{min} + \delta \leq y_r \leq p_{max}- \delta = 0.00112781\}$.
We perform reachability analysis of $M_{10}^{\delta}$ using SpaceEx \cite{frehse2011spaceex}.
Since, $M^{\delta}_{10} \models S(M^{\delta}_{10})$, we can conclude that $M_{48} \models S(M_{48})$.
\figref{BuildingModel_1} presents the reachability analysis of the full order system and its 10-order output abstraction, where for this example it was possible to compute some reachable states of the full-order system.

\begin{figure}[t!]
	\centering
		\includegraphics[width=\columnwidth]{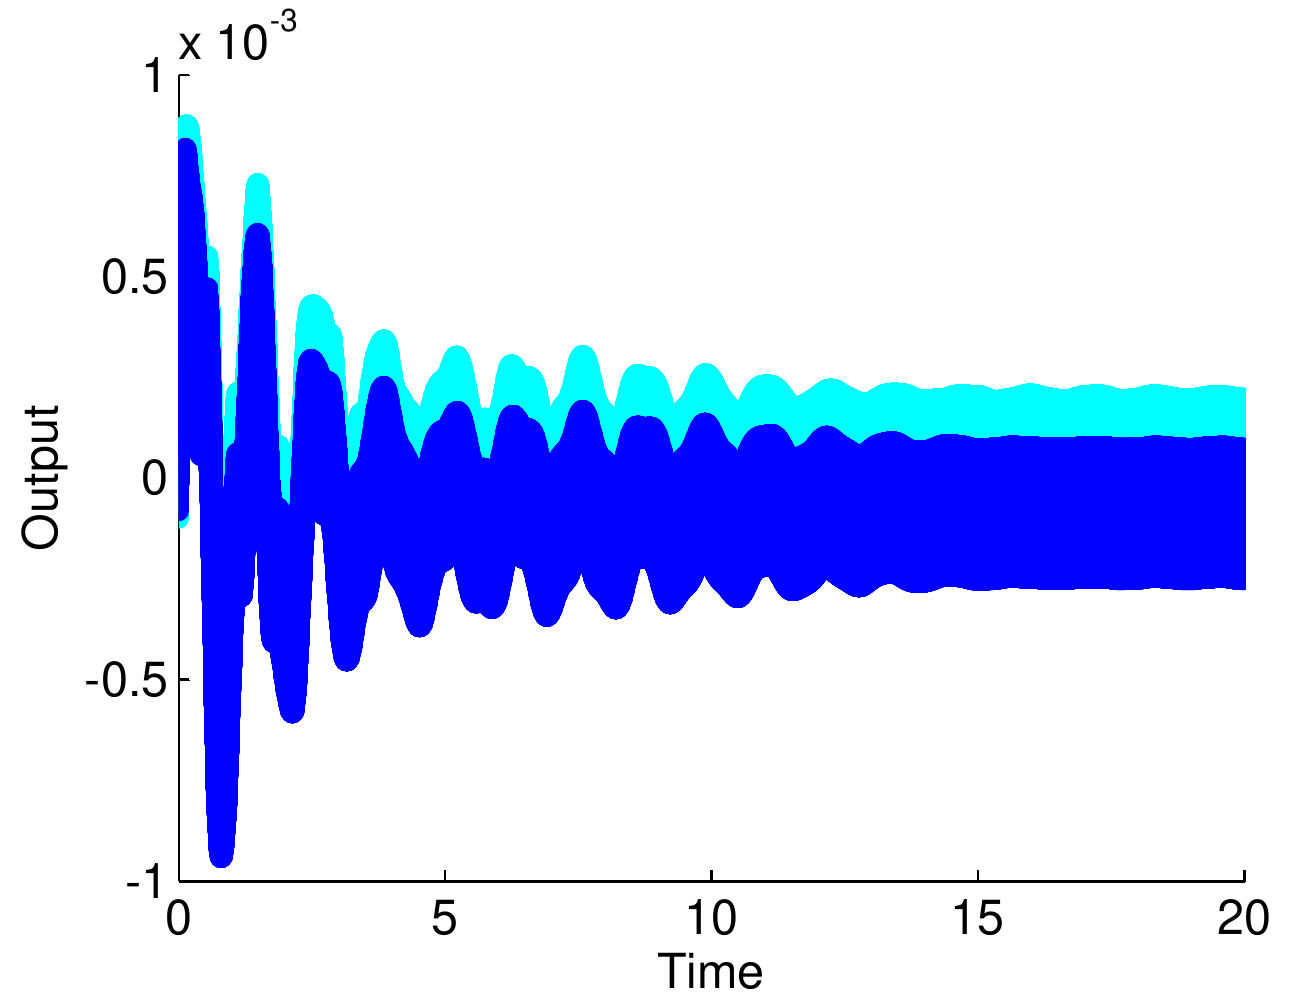}
		%\vspace{-2em}
	  \caption{Output reachability analysis of the full order BM system $M_{48}$ (cyan color) and its 10-order output abstraction $M_{10}^{\delta}$ (blue color).}
	  \figlabel{BuildingModel_1}
\end{figure}

Since we transform the original verification problem of the full order system to the new verification problem of a lower-dimensional system, the computation cost of verification process is reduced.
\figref{BuildingModel_3} illustrate the computation time and storage memory of the reachability analysis of the full order system and its output abstractions (with the time range as $[0,20s]$) using SpaceEx.
As can be seen from the figures, verification based on output abstractions can reduce significantly the computation cost especially in the time of computing reachable set.
%
%More importantly, our method is a potential approach to verify the safeness of a very high-dimensional system (with even up to a thousand of state variables) where the full order model can not be verified using the existing tools with small scalability such as SpaceEx \cite{frehse2011spaceex}, Flow* \cite{chen2013flow} and dReach \cite{kong2015dreach}.

\begin{figure}[t!]%
    \centering%
		\begin{subfigure}[t]{0.49\columnwidth}%
			\centering%
			\includegraphics[width=\linewidth]{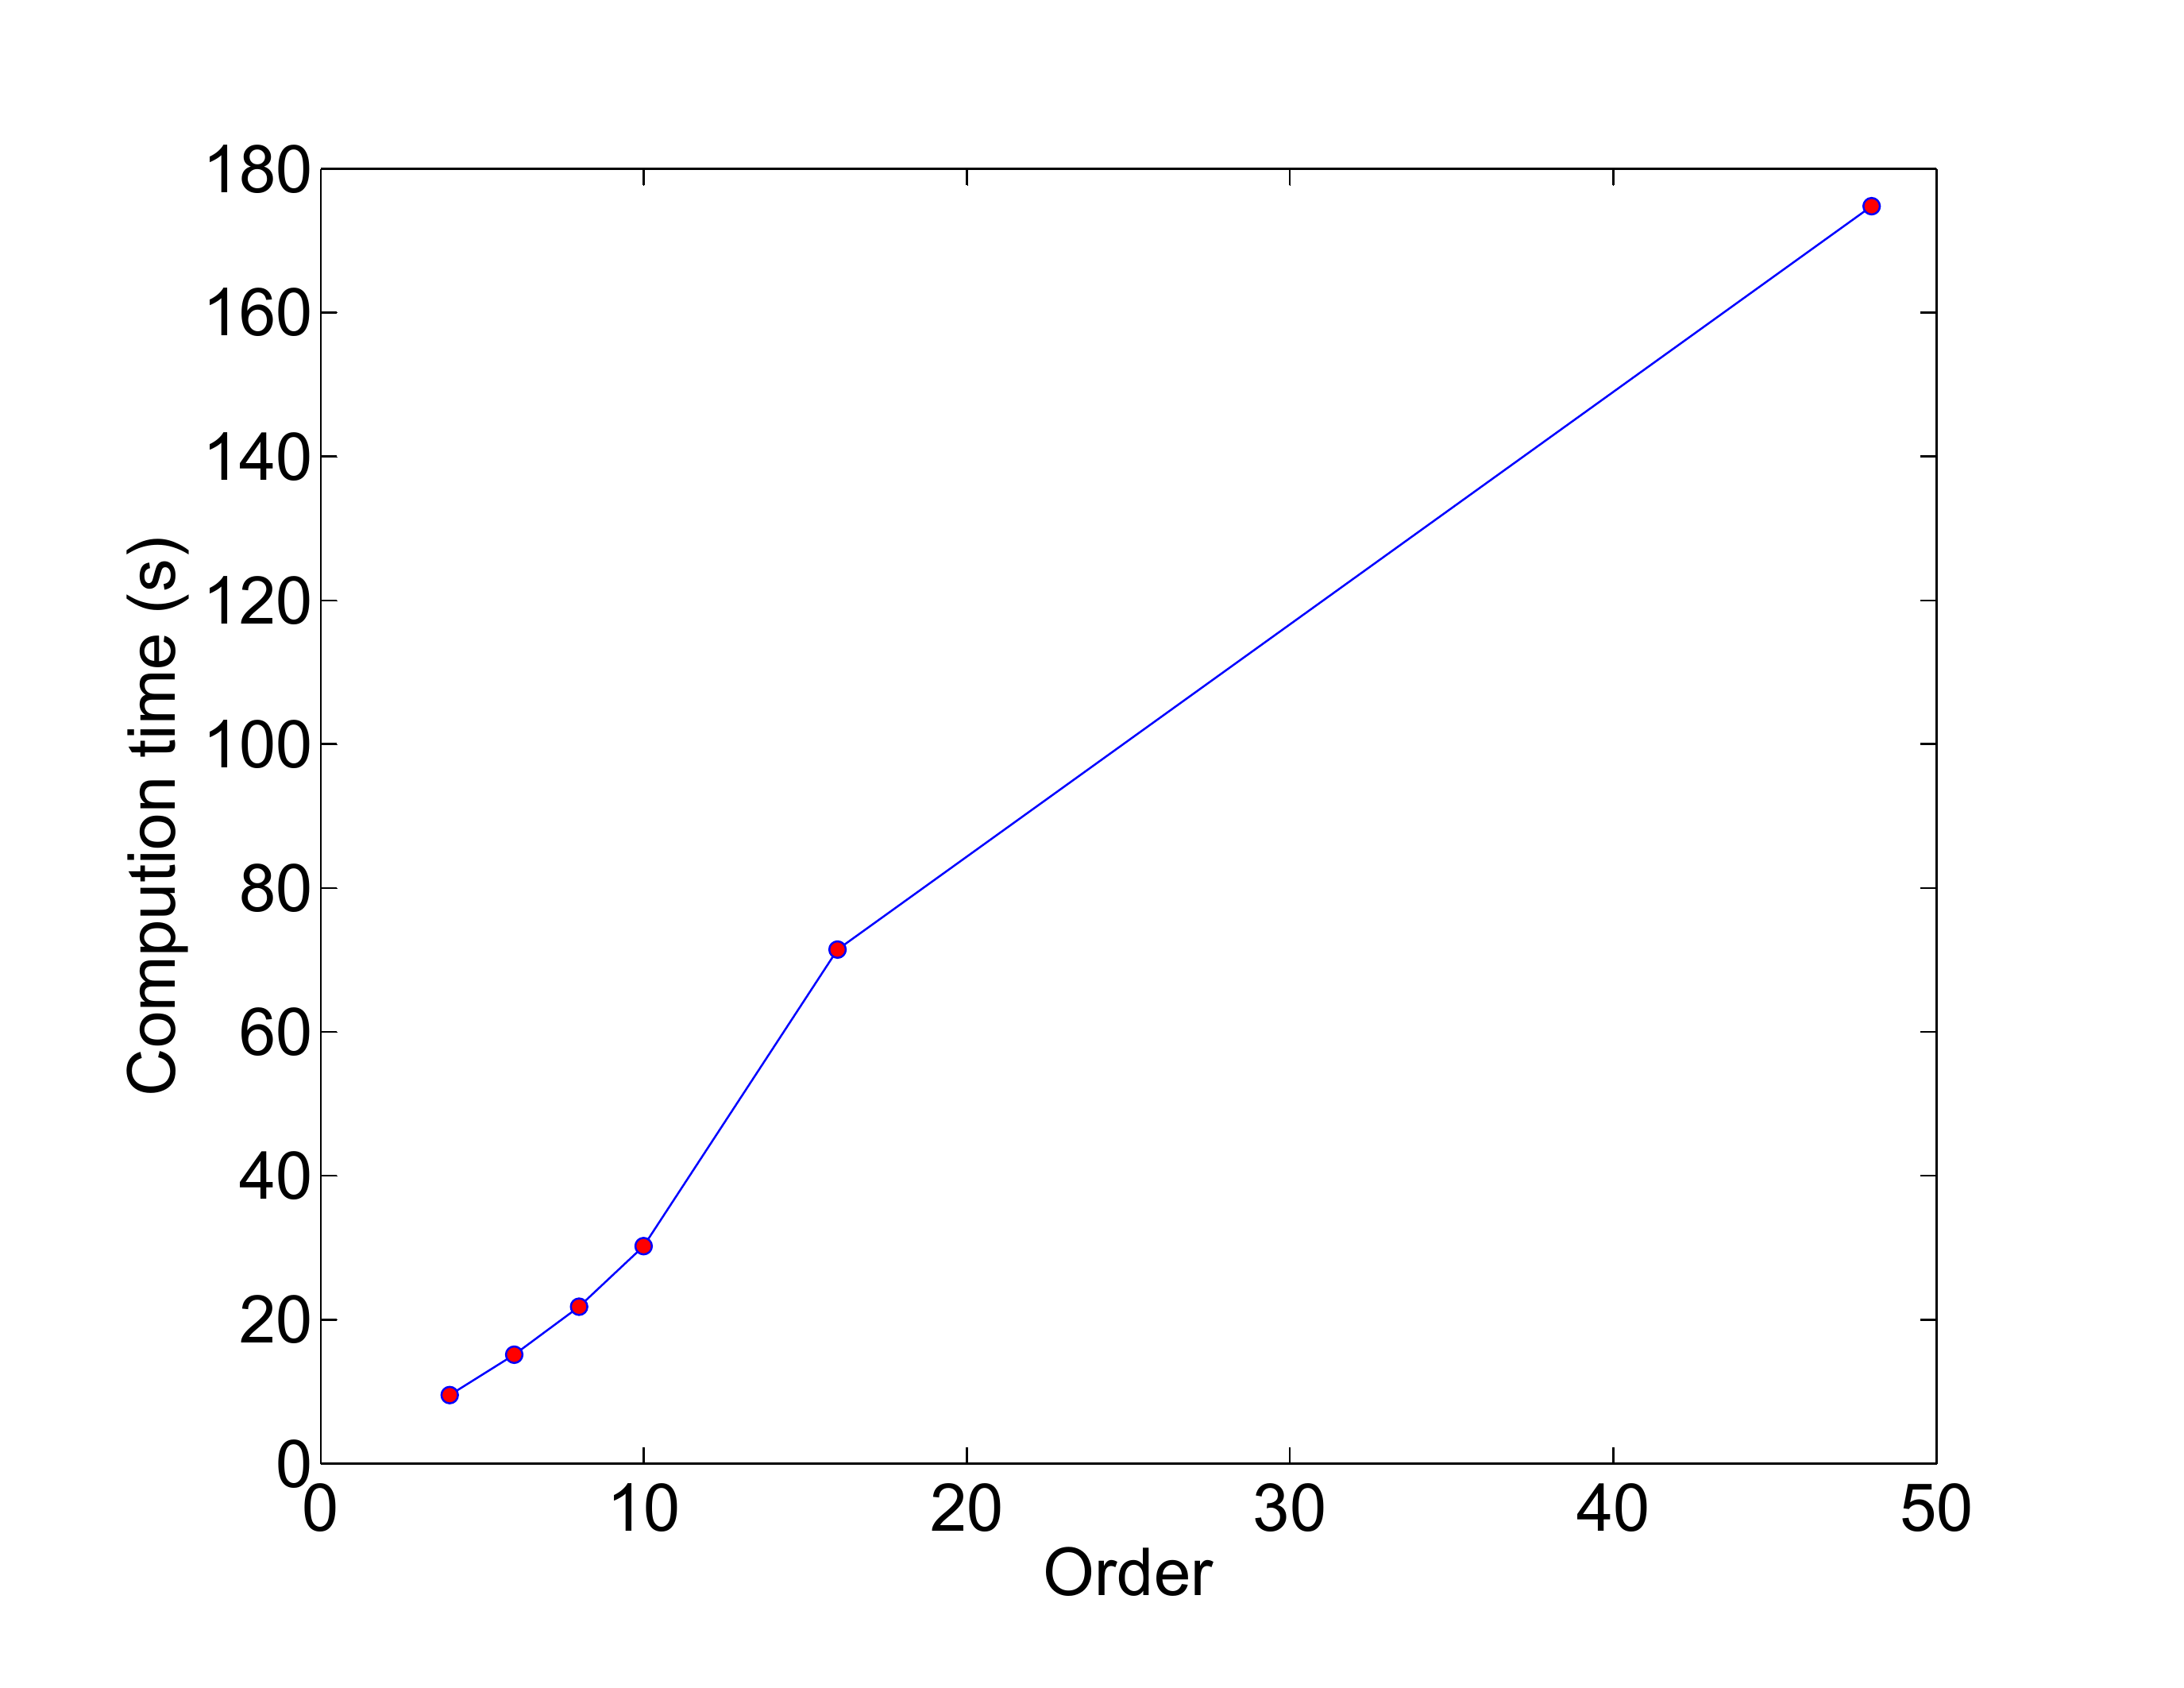}
			%\caption{}%
			\figlabel{vanderpol_streamplot}%
		\end{subfigure}%
~
    \begin{subfigure}[t]{0.49\columnwidth}%
				\centering%
				\includegraphics[width=\linewidth]{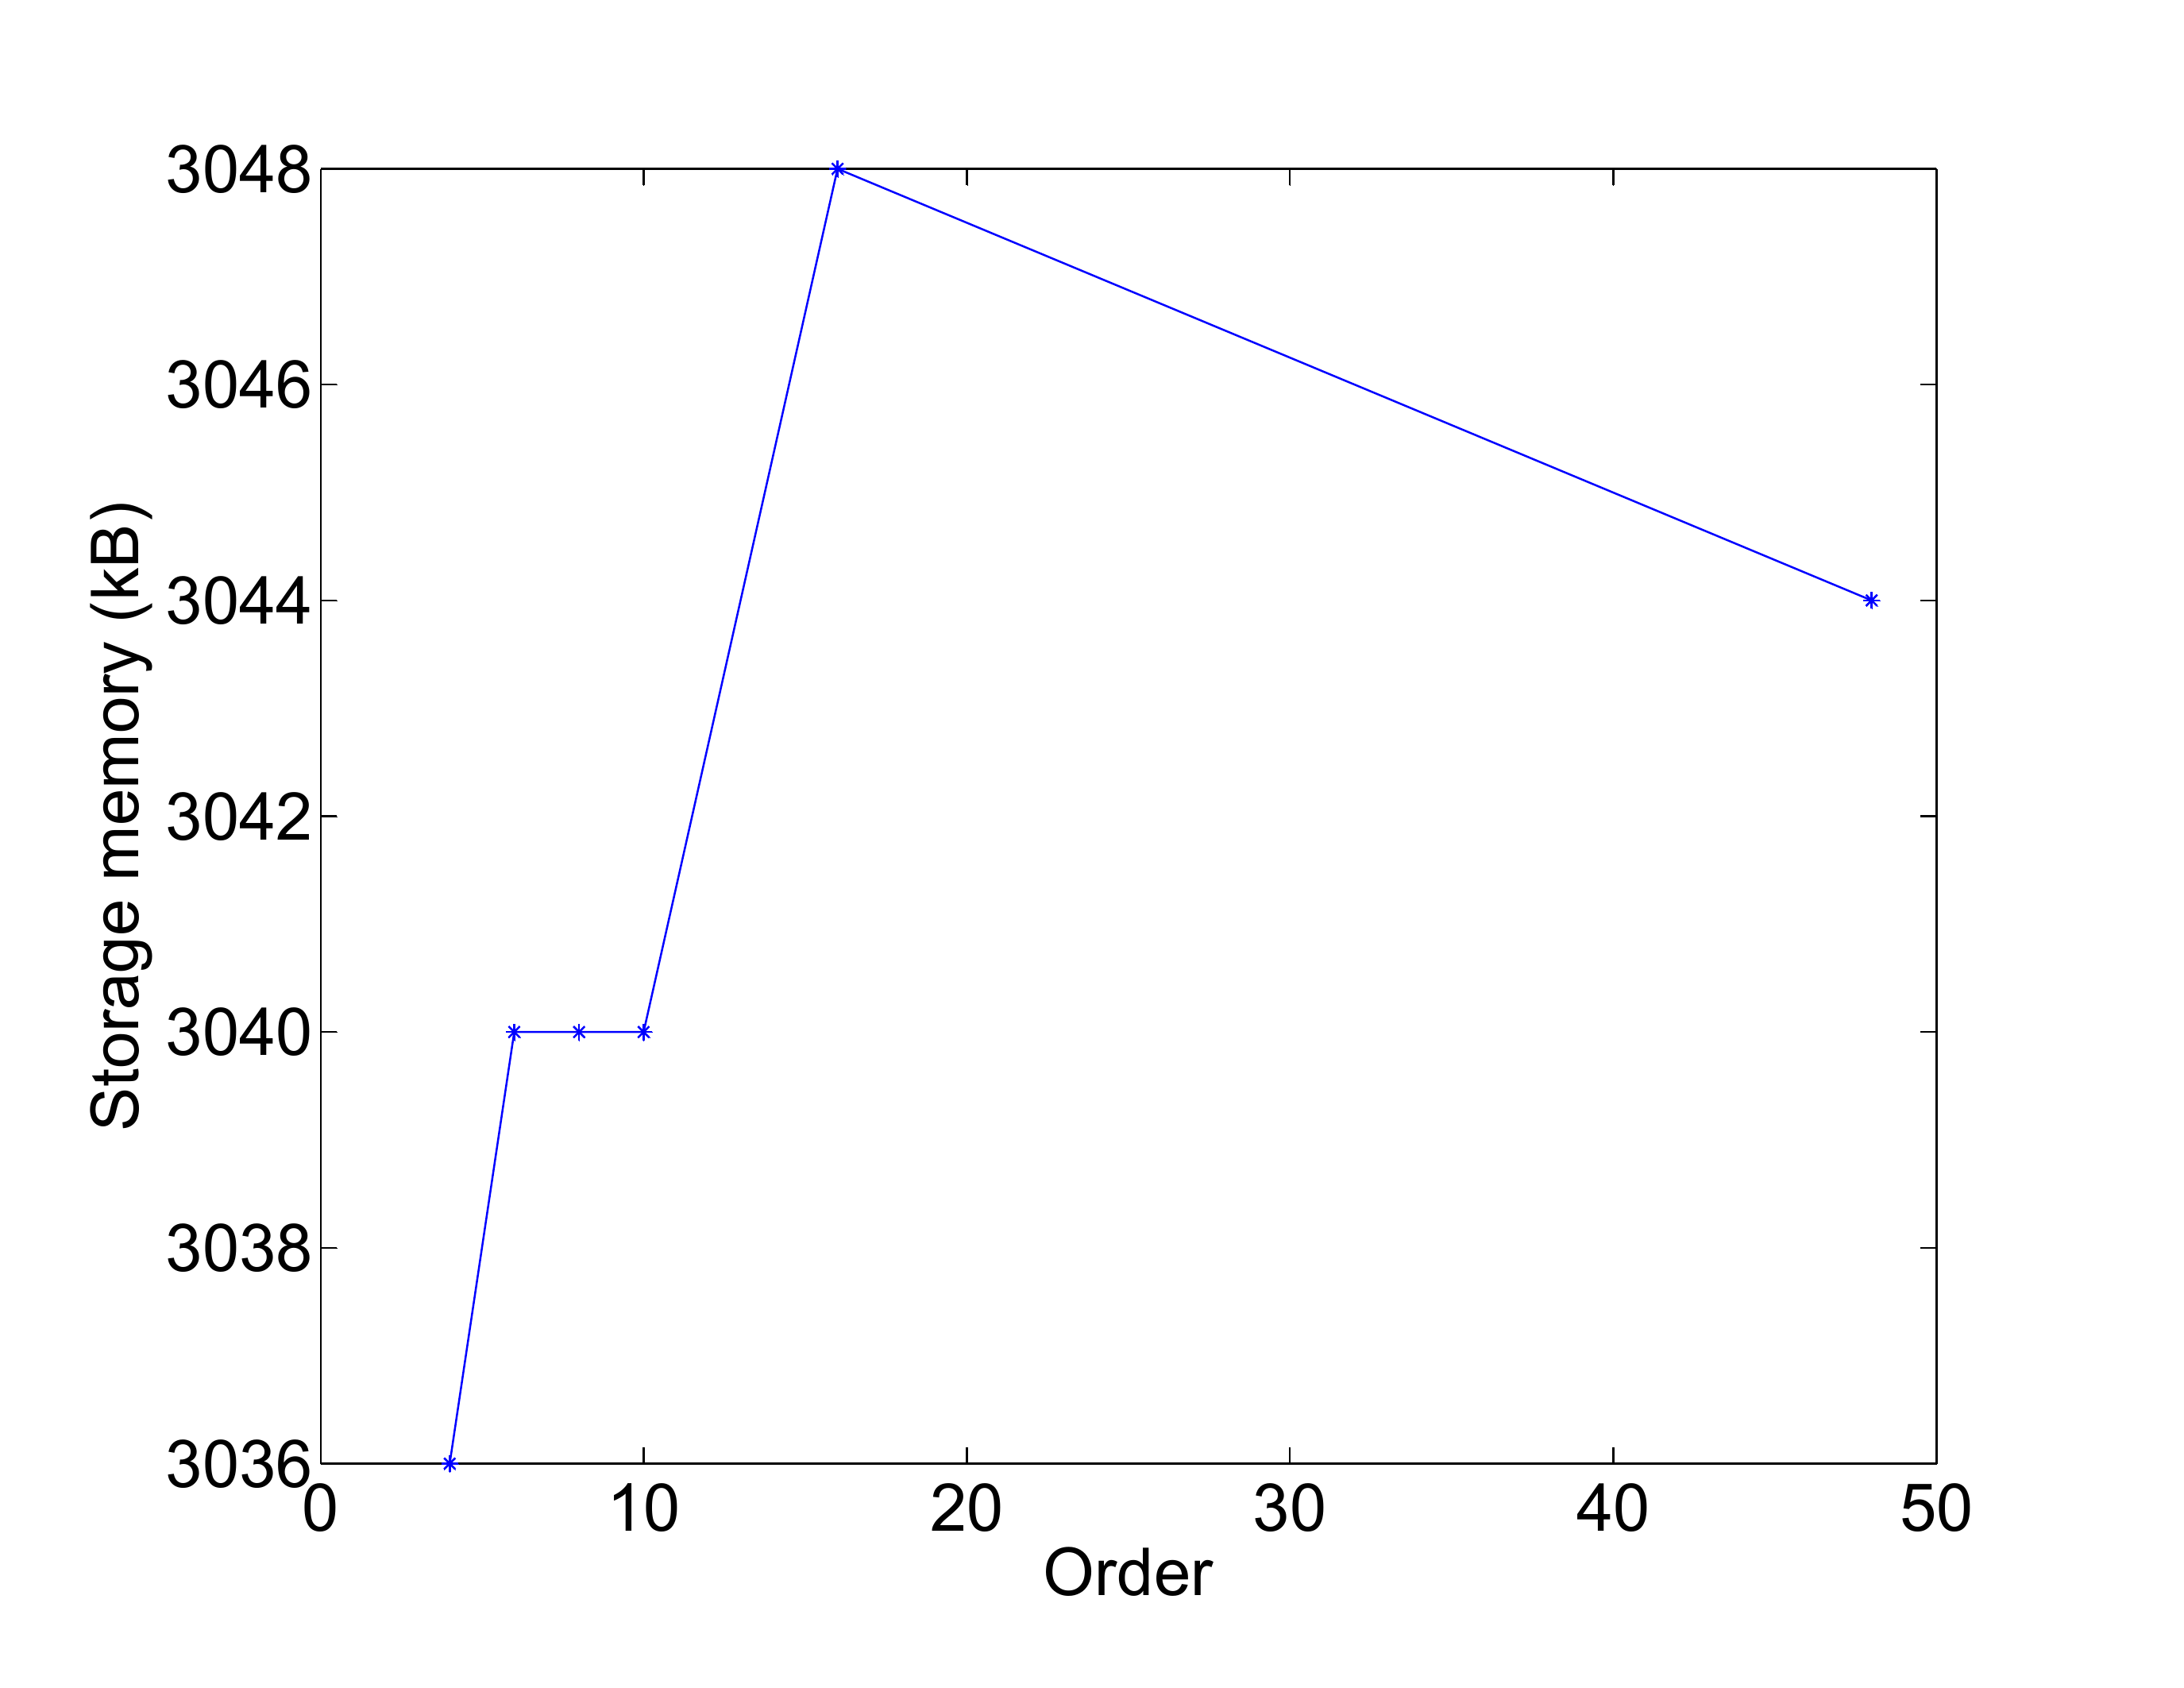}
				%\caption{}%
				\figlabel{vanderpol_reach}%
    \end{subfigure}%
    \caption{Reachable set computation time (left) and storage memory (right) versus the orders of different output abstractions.}%
		\figlabel{BuildingModel_3}%
		%\vspace{-1.25em}%
\end{figure}%

As we can see above, there exist many different output abstractions that can be used to verify the safeness of the original system $M_{48}$.
The lower-dimensional output abstraction is used, the lower computation cost can be achieved.
Thus, seeking the lowest-dimensional output abstraction is one of the most important task in our approach.
Applying the semi-algorithm from~\figref{algorithm}, the 4-order output abstraction is given as the lowest-dimensional one that can be used to verify the safety requirement of the original system.
Its error bound $\delta$ is equal to $4.2784e-04$ and its matrices are as follows,
\begin{equation*}
\begin{split}
&A = \begin{bmatrix} -0.0075 & 5.2756 & -0.0010 &-0.6634 \\ -5.2756 & -0.8574 & 0.0904 & 0.9217  \\ -0.0010 & -0.0904 & -0.0001 & -13.5419 \\  0.6634 & 0.9217 & 13.5419 & -1.0040 \\ \end{bmatrix}, \\
&B = \begin{bmatrix}  0.0061 & 0.0645 & 0.0007 & -0.0622 \\\end{bmatrix}^T, \\
&C = \begin{bmatrix}-0.0061 & 0.0645  & -0.0007 & -0.0622 \\ \end{bmatrix}.
\end{split}
\end{equation*}

The transformed initial set of the 4-order output abstraction is given in the same form as $X_0(M_{10}^{\delta})$ in which the lower bound and upper bound vectors are presented in \tabref{tab:3}.

\begin{table}
	\centering
	\begin{tabular}{|l|l|}
  \hline
  Vector  & Value \\
	\hline
  $lb_r$  & [-0.0448e-03~~-0.4711e-03~~-0.0051e-03~~-0.4543e-03$]^T$  \\
  $ub_r$  & [0.0448e-03~~0.4711e-03~~0.0051e-03~~0.4543e-03$]^T$  \\
  $a$     & -5.8951e-05 \\
	$b$     &  5.8951e-05  \\
  \hline
\end{tabular}
	\caption{Transformed initial condition of the BM's 4-order output abstraction $M_{4}^{\delta}$.}
	\tablabel{tab:3}
\end{table}

\figref{BuildingModel_4} shows the error bounds of the output abstractions while \figref{BuildingModel_5} illustrates the comparison between the output bounds $||y_r||$ of the output abstractions $M_k^{\delta}$ and its transformed safety specification $S(M_k^{\delta})$.
As shown in~\figref{BuildingModel_4}, the bound of zero-input response error $e_1$ increases along with the order of the output abstraction while the bound of zero-state response error $e_2$ fluctuates but generally decreases along with the order of the output abstraction.
This leads to the decrease with fluctuation of the error bound $\delta$ which causes an interesting problem that the 5, 7, 9-order output abstractions do not satisfy their transformed safety specifications while the 4, 6, 8-order output abstractions do as shown in~\figref{BuildingModel_5}.
It is emphasized that when an output abstraction's satisfaction of the transformed safety specification is indeterminate, we can conclude nothing about the safety of the original system.

\begin{figure}[t!]
	\centering
		\includegraphics[width=\columnwidth]{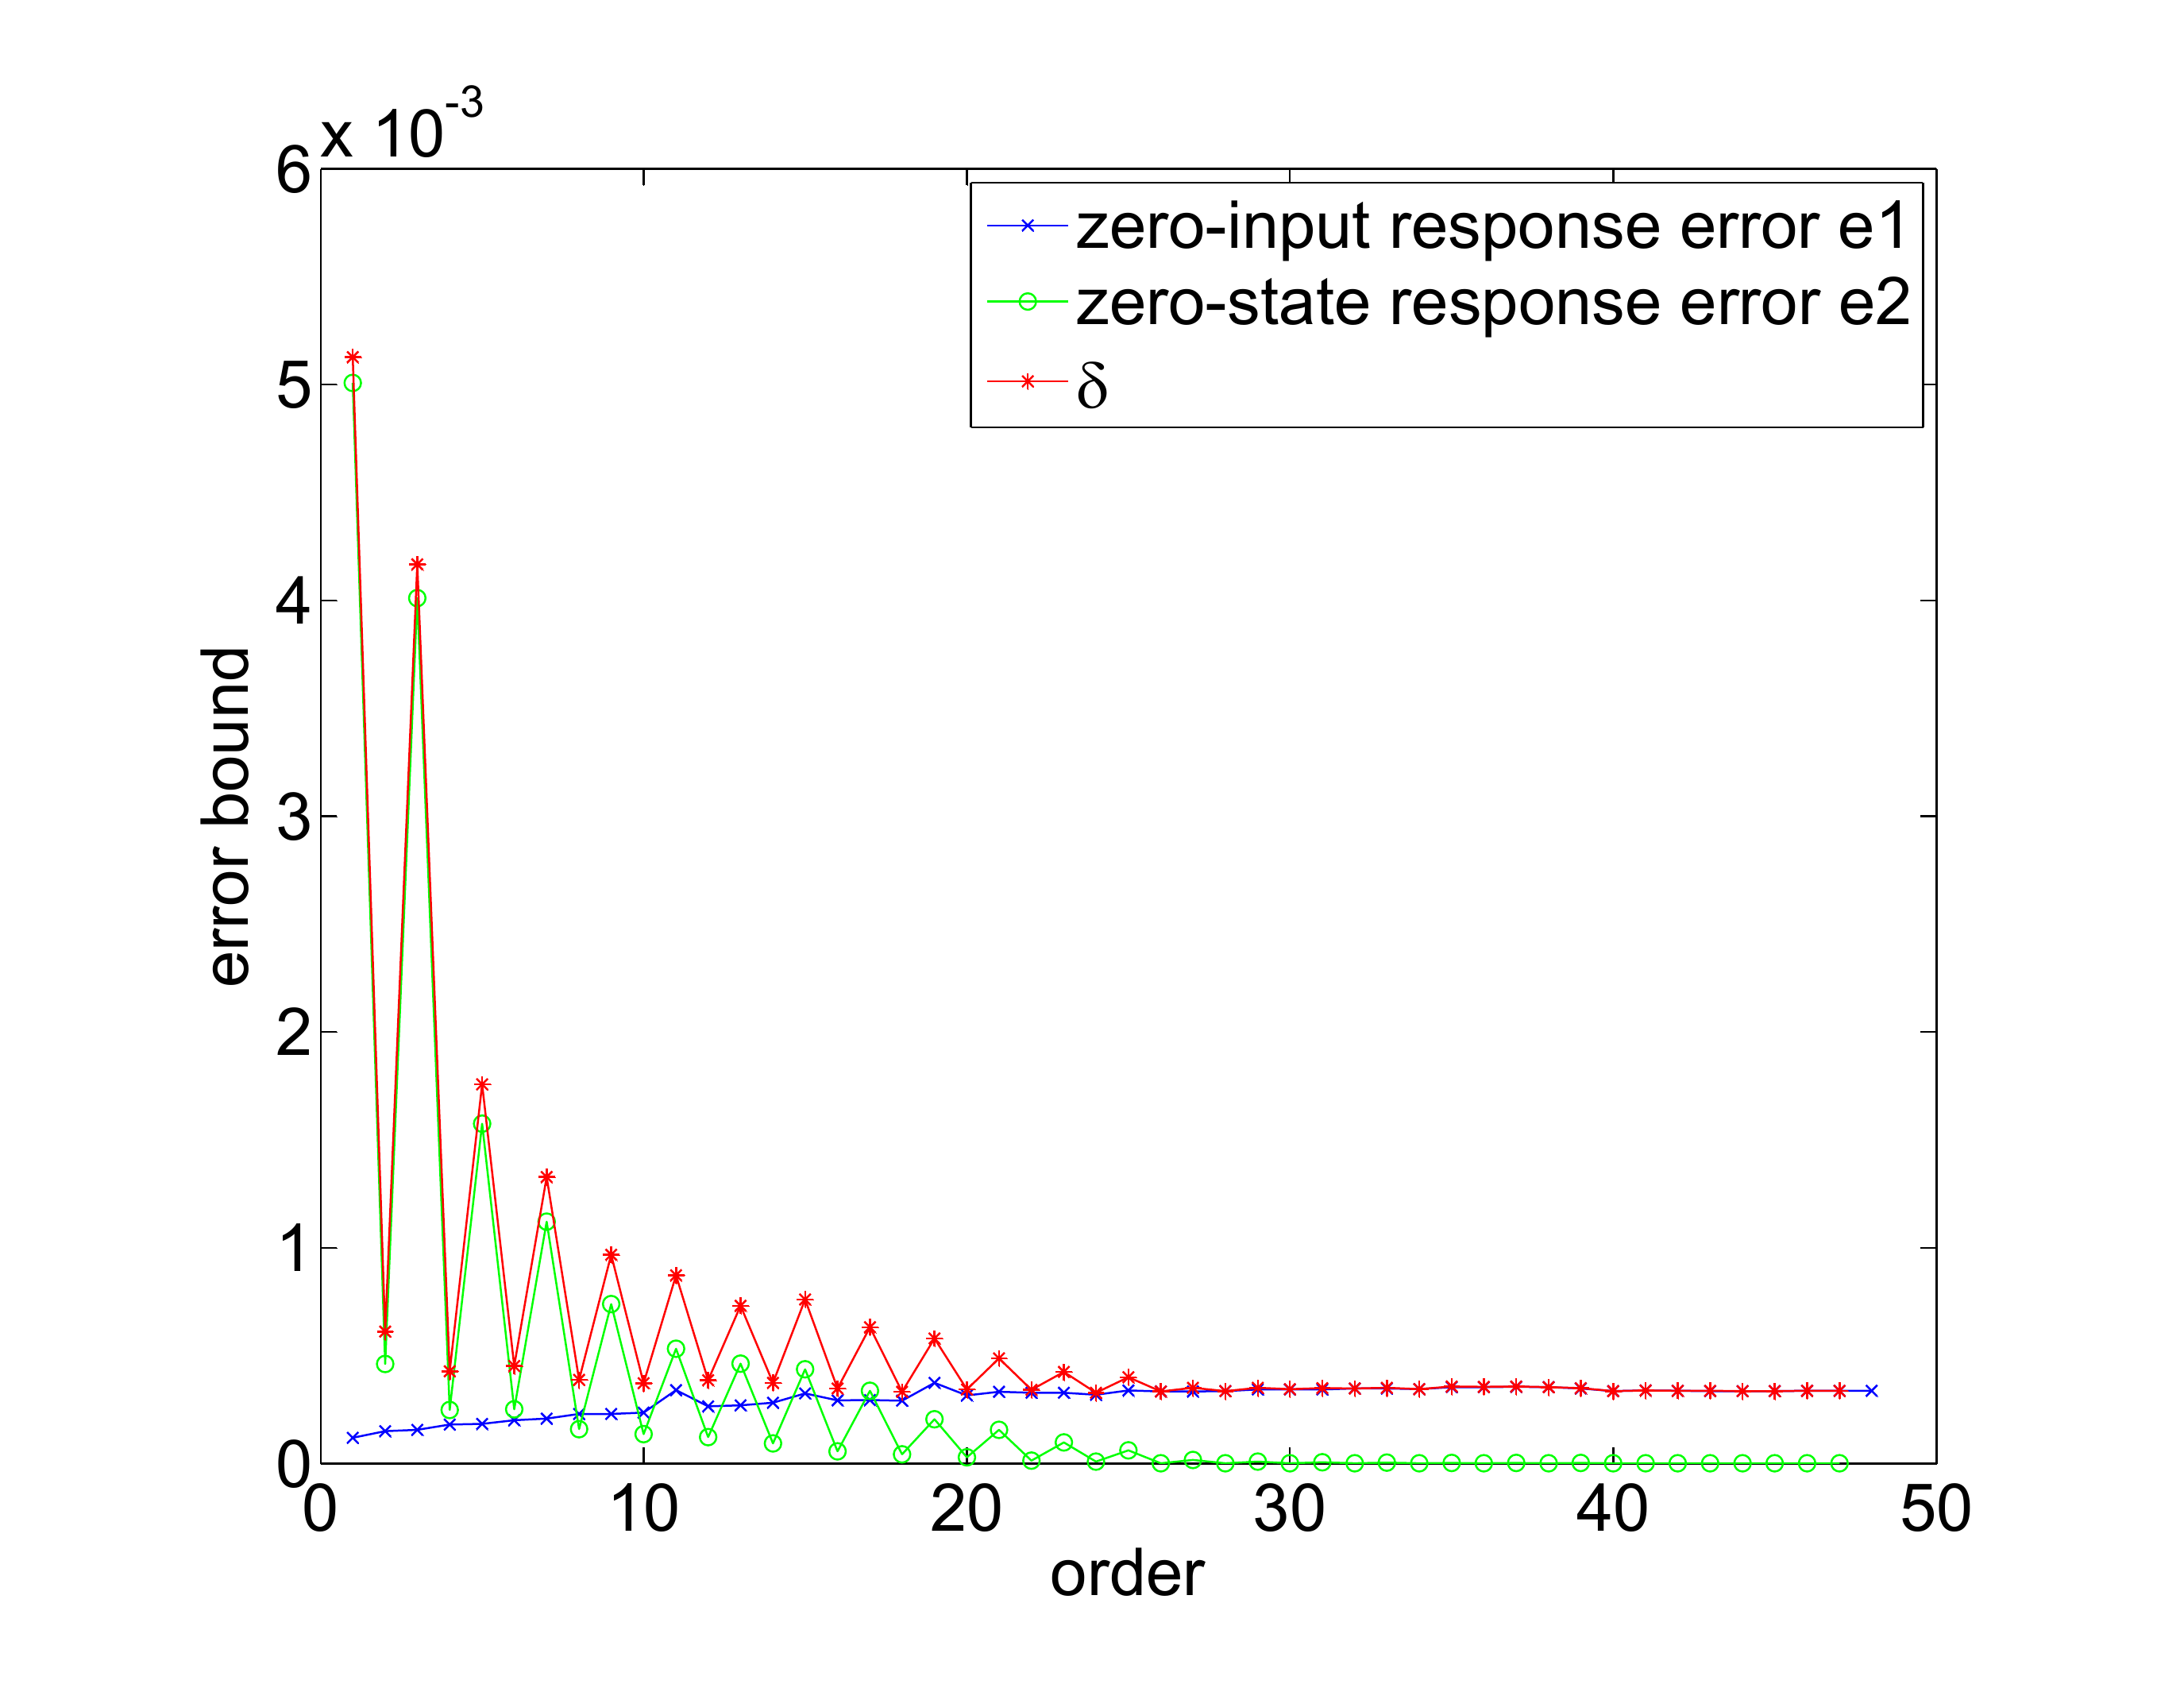}
	  \caption{Error bounds (zero-input response error $e_1$, zero-state response error $e_2$ and the total error bounds $\delta$) between the full order BM system and its output abstraction versus the orders of different abstractions.}
	  \figlabel{BuildingModel_4}
\end{figure}

\begin{figure}[t!]
	\centering
		\includegraphics[width=\columnwidth]{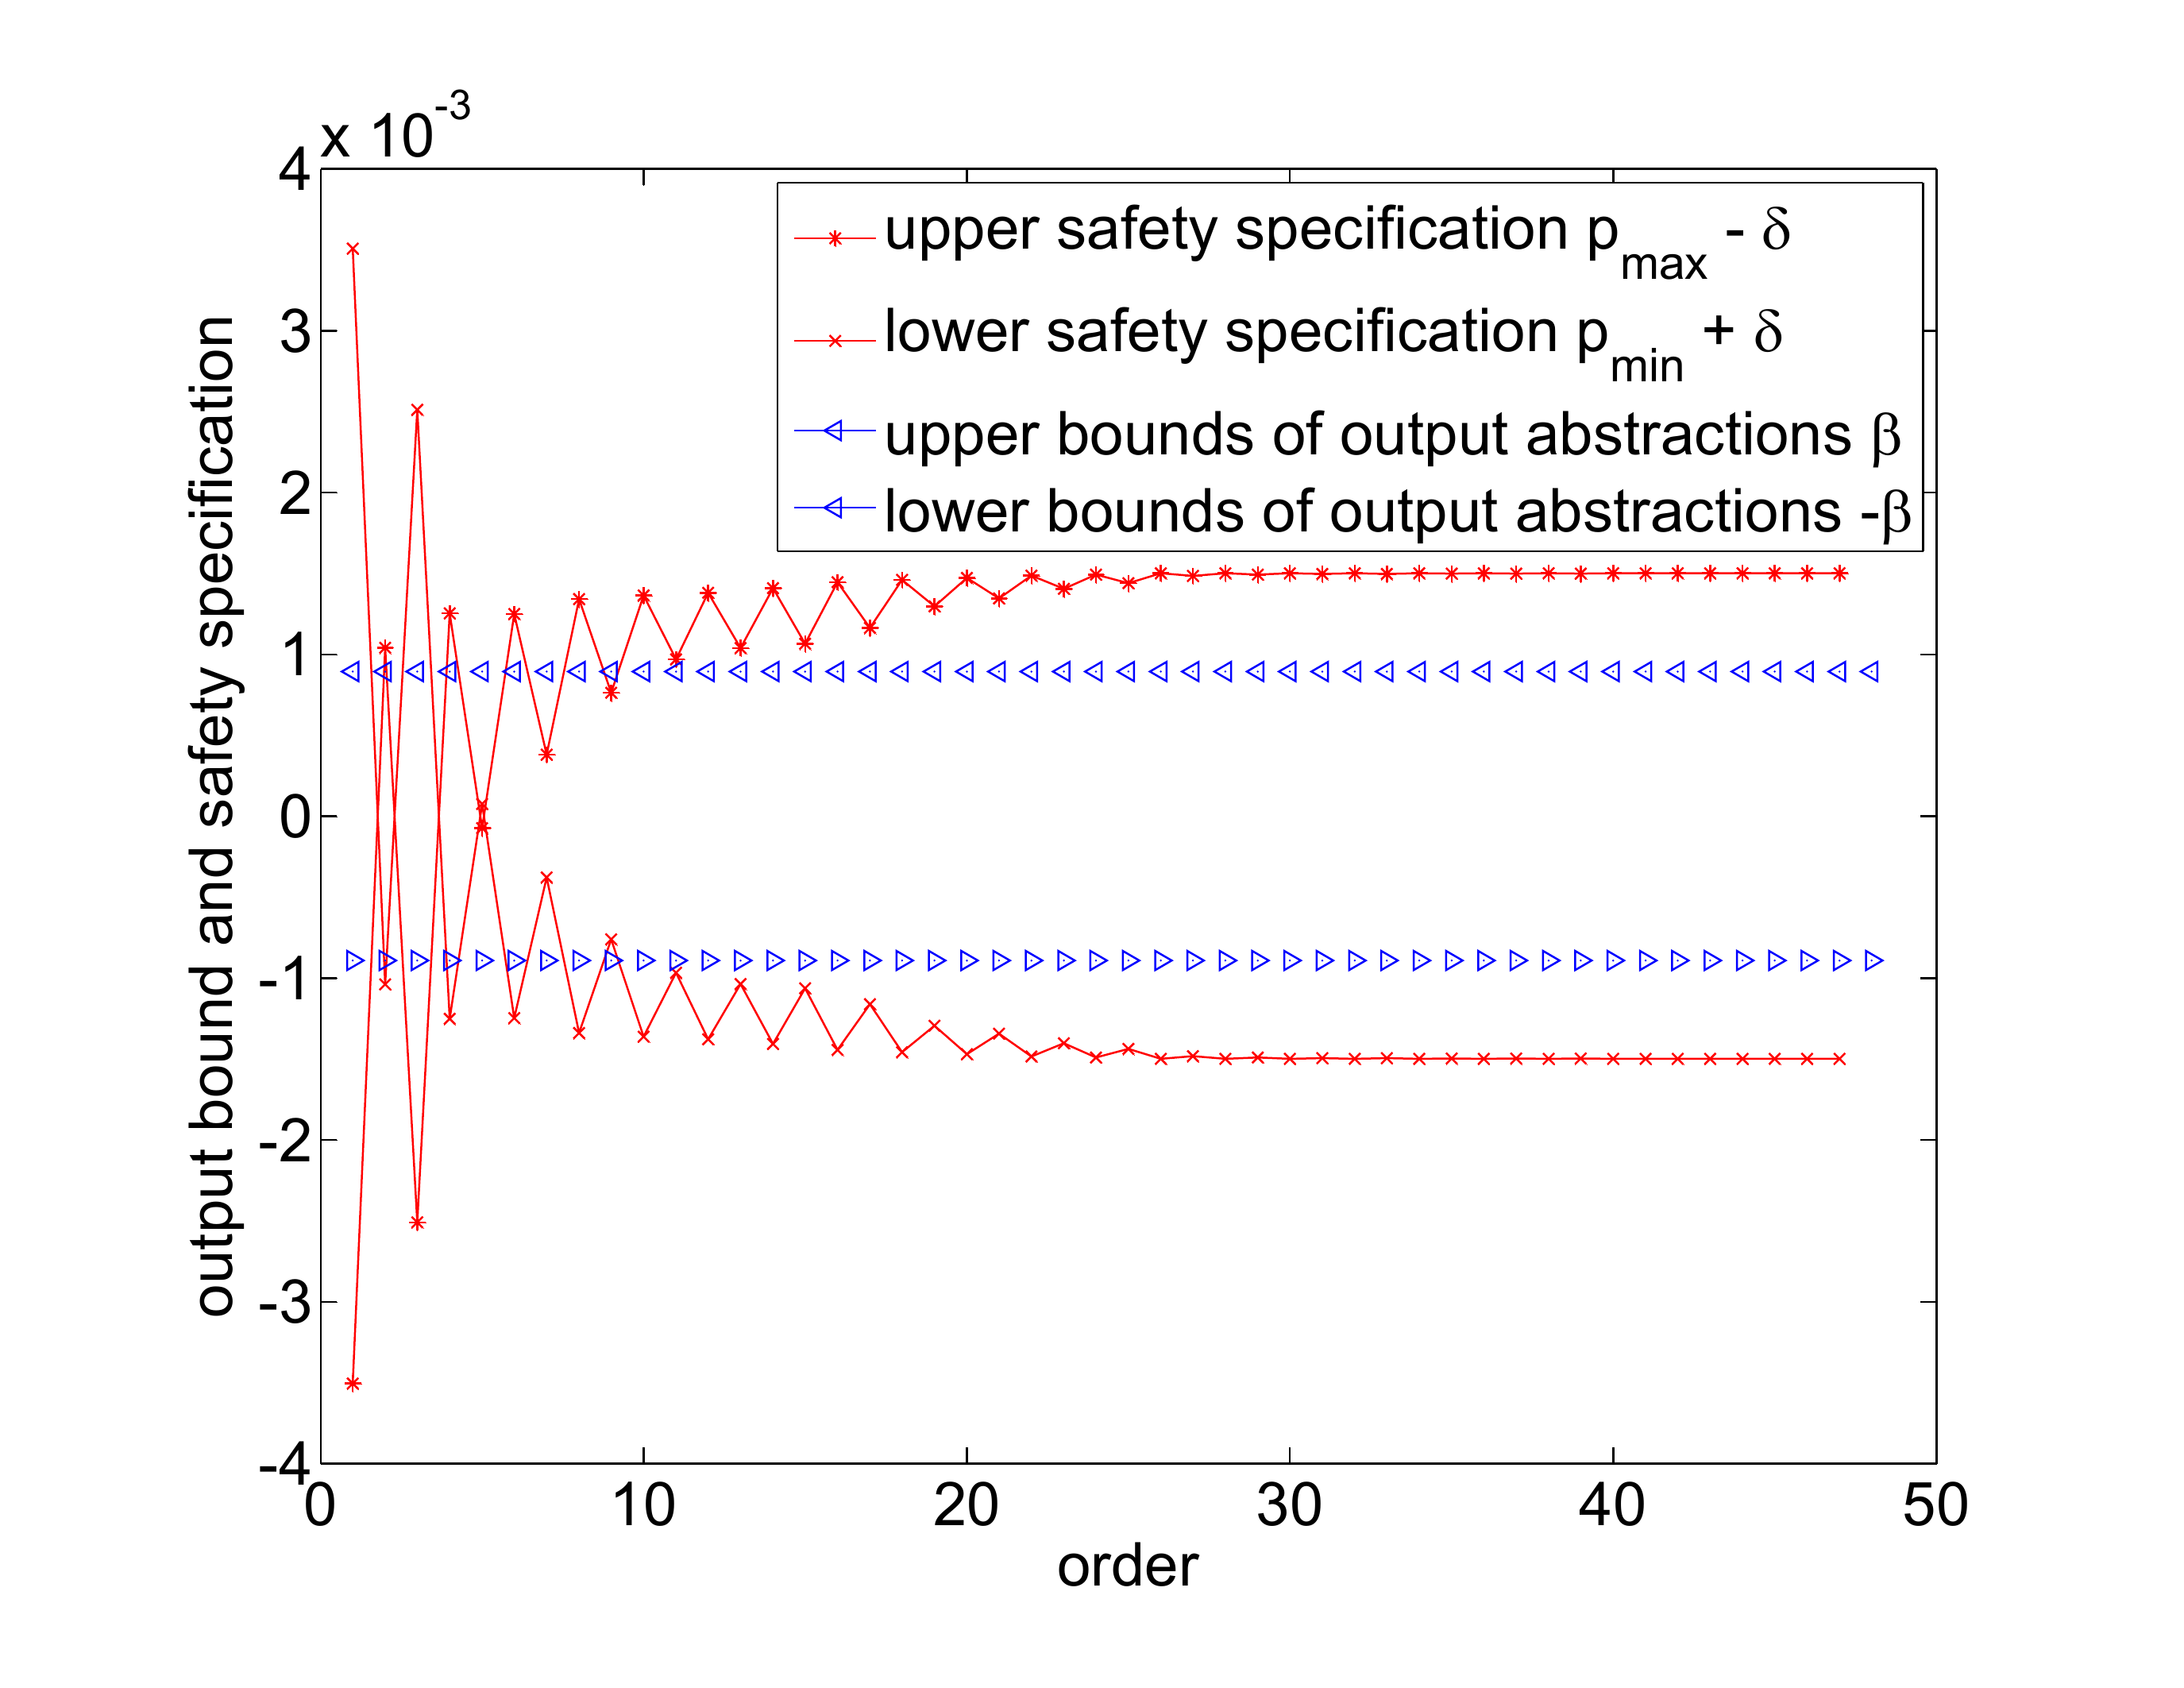}
	  \caption{Output bounds and the corresponding transformed safety specifications versus the orders of different output abstractions.}
	  \figlabel{BuildingModel_5}
\end{figure}
